# Supplementary material for: Trends in the hyperfine interactions of magnetic adatoms on thin insulating layers
Source: arXiv:2012.11639 ancillary file (2020-12-21)
Supplement: Supplementary file 1 [file SI.pdf]

# Supplementary Material for "Trends in the hyperfine interactions of magnetic adatoms on thin insulating layers"

Sufyan Shehada,[1,2,*] Manuel dos Santos Dias,[1] Filipe Souza Mendes Guimarães,[1] Muayad Abusaa,[3] and Samir Lounis[1,4]

[1]*Peter Grünberg Institut and Institute for Advanced Simulation, Forschungszentrum Jülich and JARA, 52425 Jülich, Germany*

[2]*Department of Physics, RWTH Aachen University, 52056 Aachen, Germany*

[3]*Department of Physics, Arab American University, Jenin, Palestine*

[4]*Faculty of Physics, University of Duisburg-Essen, 47053 Duisburg, Germany*

(Dated: December 21, 2020)

* s.shehada@fz-juelich.de

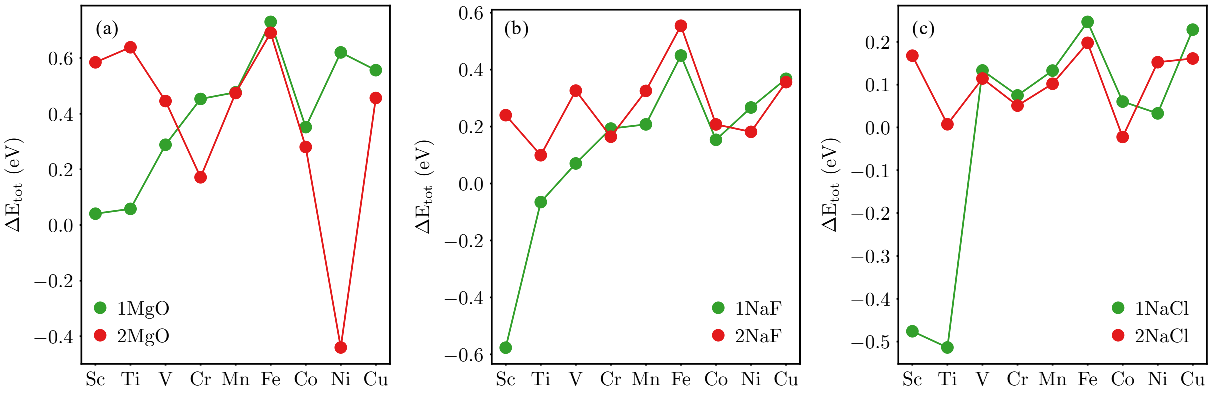


FIG. 1. Total energy of adatoms on the bridge position relative to the one for the anion-top position energy, calculated for structures relaxed within GGA-PBE. Ultra-thin films: (a) MgO, (b) NaF and (c) NaCl. The number to the left of the chemical formula in the legend indicates the number of layers in the ultra-thin film.

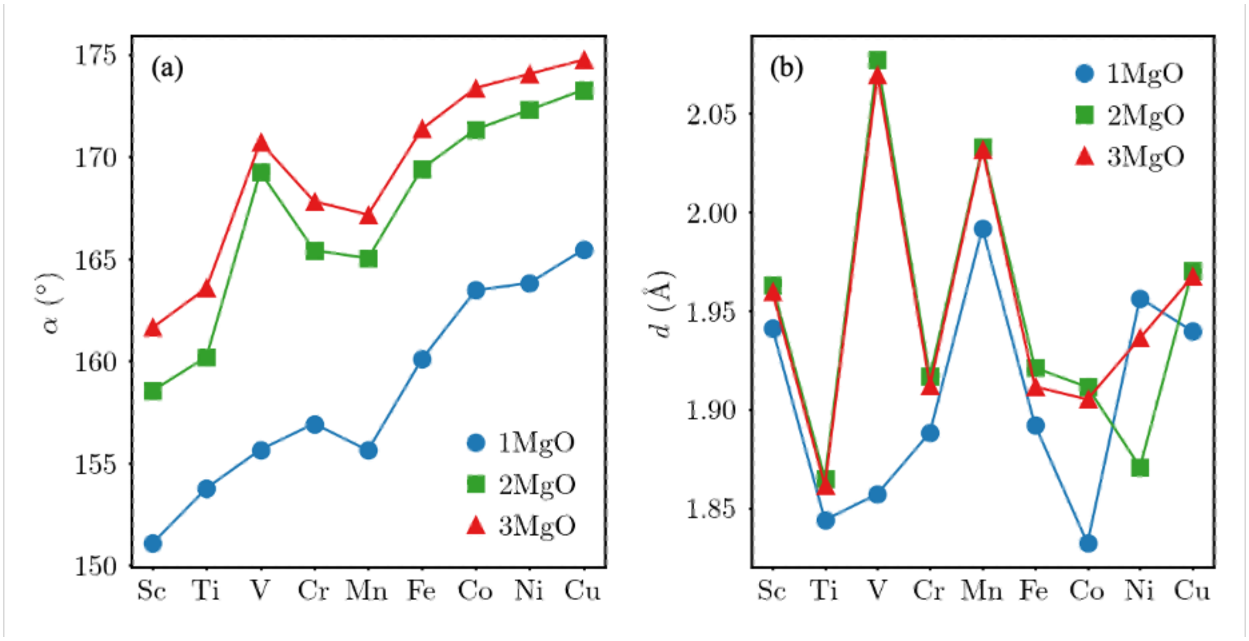


FIG. 2. Relaxed geometrical properties of adatoms on MgO ultra-thin films, placed on top of oxygen. (a) Mg-O-Mg bond angle and (b) Distance between the adatom and oxygen. The number to the left of the chemical formula in the legend indicates the number of layers.

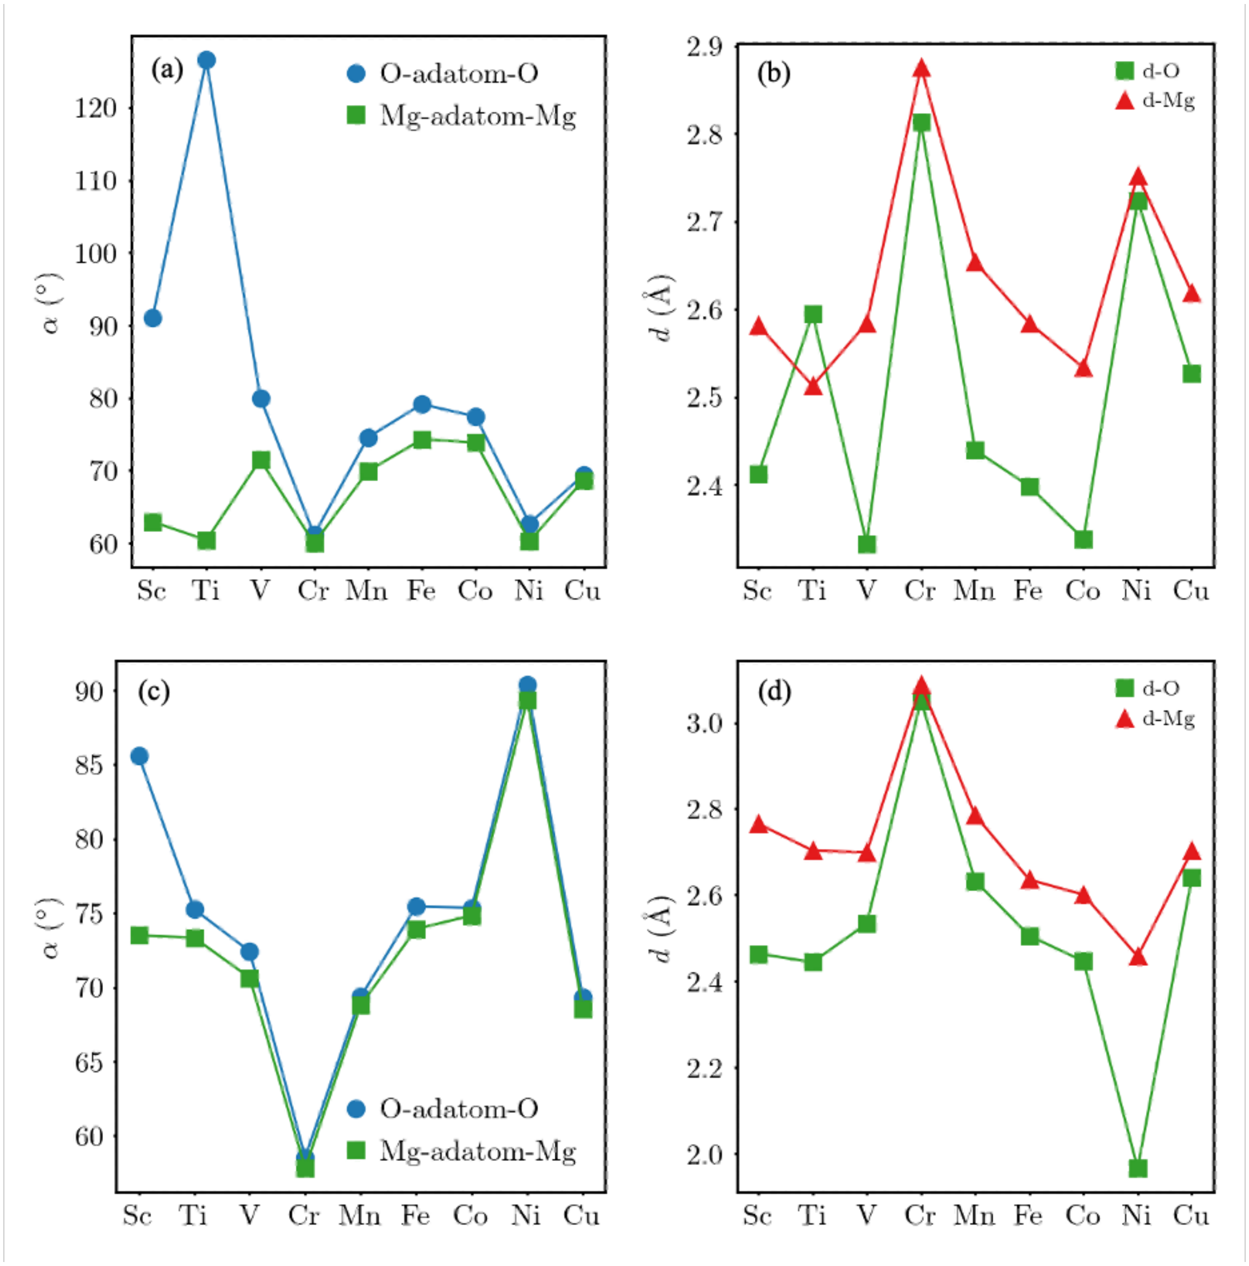


FIG. 3. Relaxed geometrical properties of adatoms on MgO ultra-thin films, placed on the bridge position. (a,c) Mg–adatom–Mg and O–adatoms–O bond angle and (b,d) Distance between the adatom and Mg and O. (a,b) results for single layer and (c,d) results for two layers of MgO.

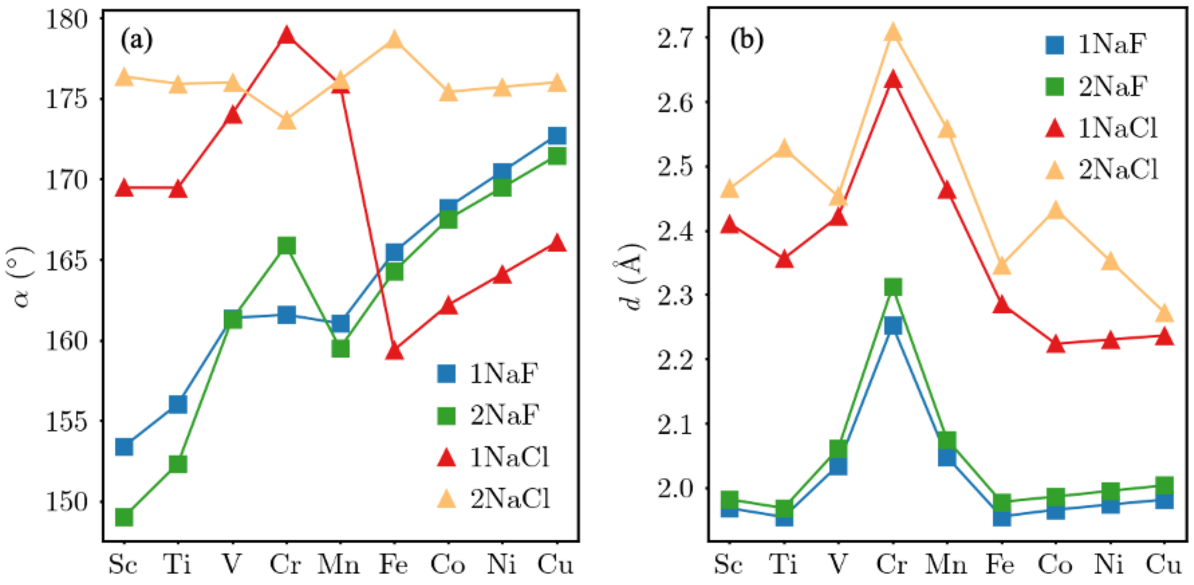


FIG. 4. Relaxed geometrical properties of adatoms on NaF and NaCl ultra-thin films, placed on top of the respective anion. (a) Na–F–Na or Na–Cl–Na bond angle and (b) distance between the adatom and either F or Cl. The number to the left of the chemical formula in the legend indicates the number of layers.

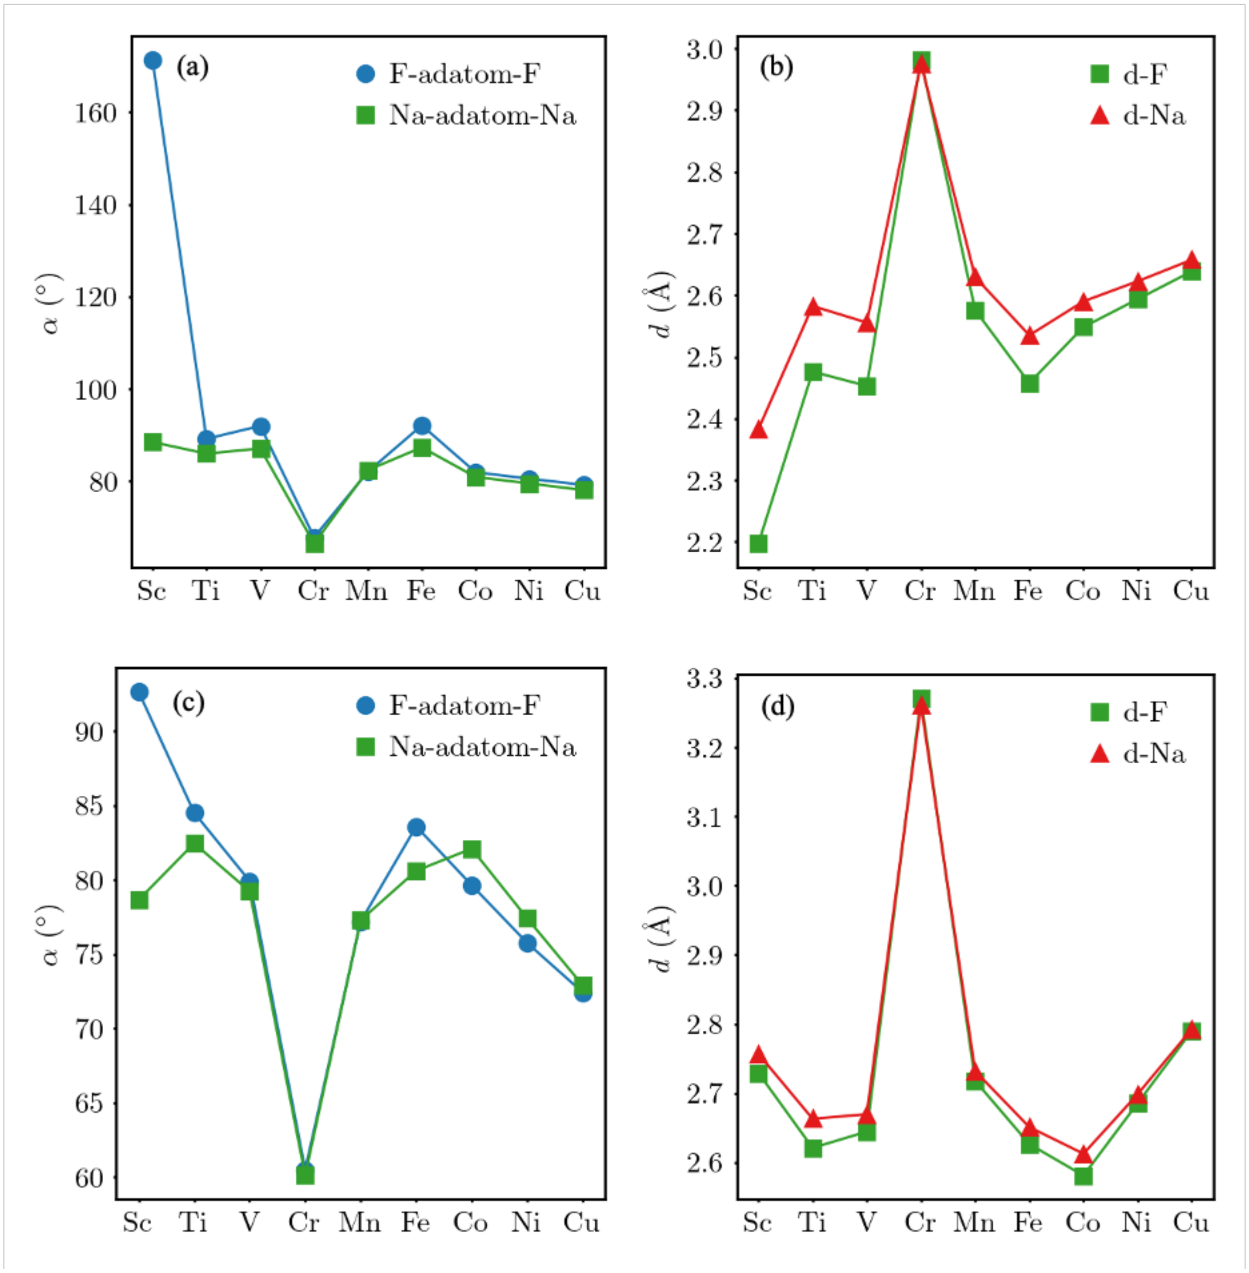


FIG. 5. Relaxed geometrical properties of adatoms on NaF ultra-thin films, placed on the bridge position. (a,c) F–adatom–F and Na–adatom–Na bond angle, (b,d) Distance between the adatom and either F or Na. (a,b) results for single layer and (c,d) results for two layers of NaF.

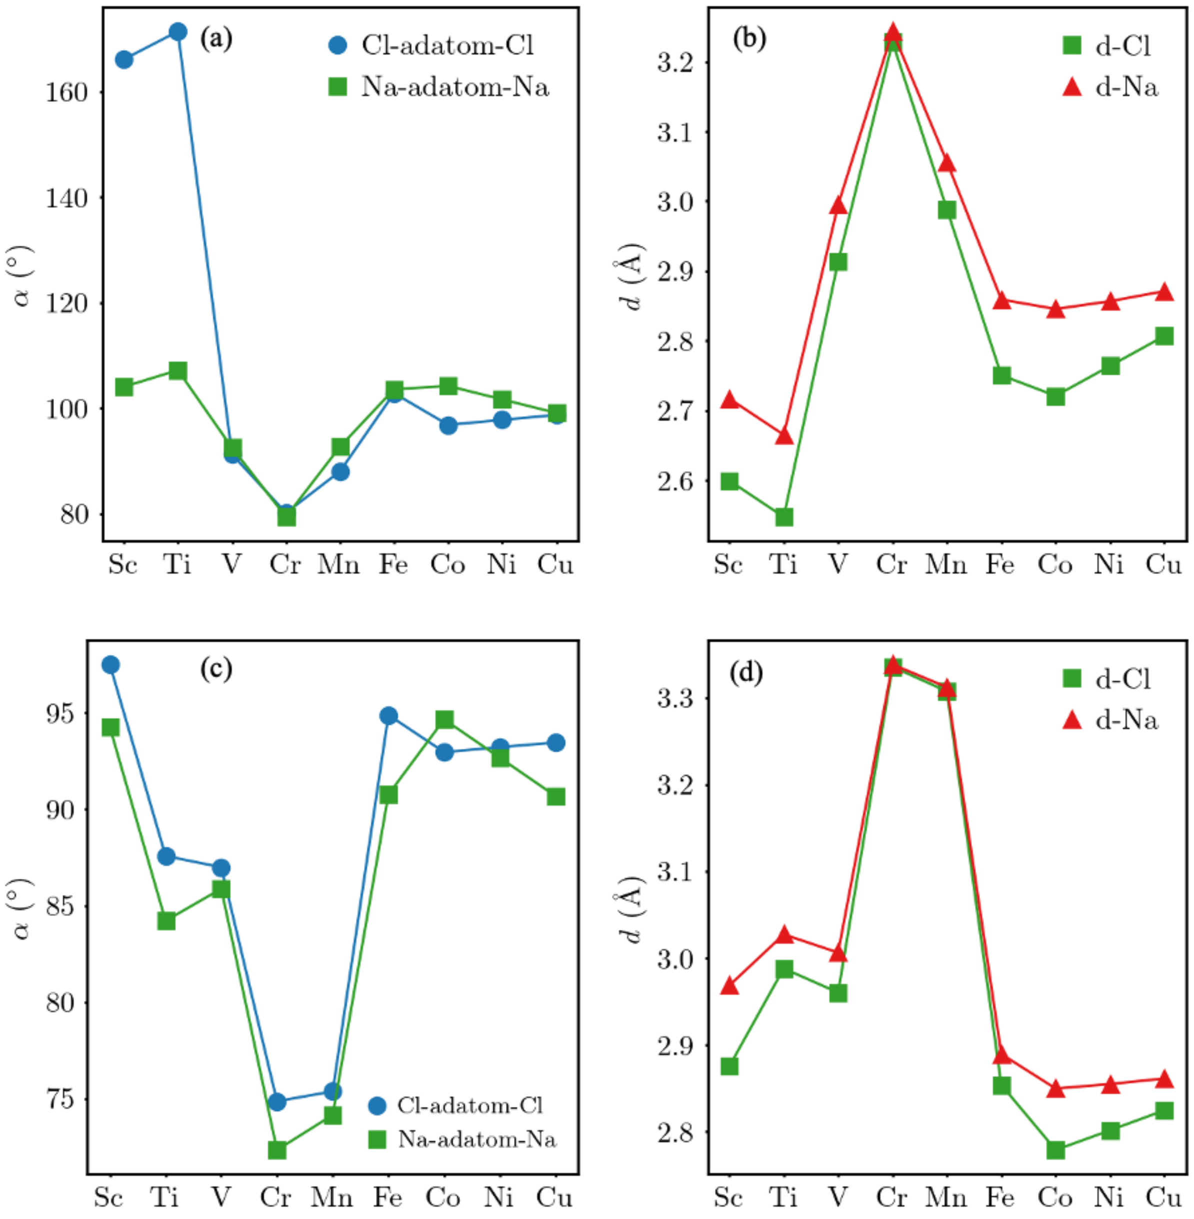


FIG. 6. Relaxed geometrical properties of adatoms on NaCl ultra-thin films, placed on the bridge position. (a,c) Cl–adatom–Cl and Na–adatom–Na bond angle, (b,d) Distance between the adatom and either Cl or Na. (a,b) results for single layer and (c,d) results for two layers of NaCl.

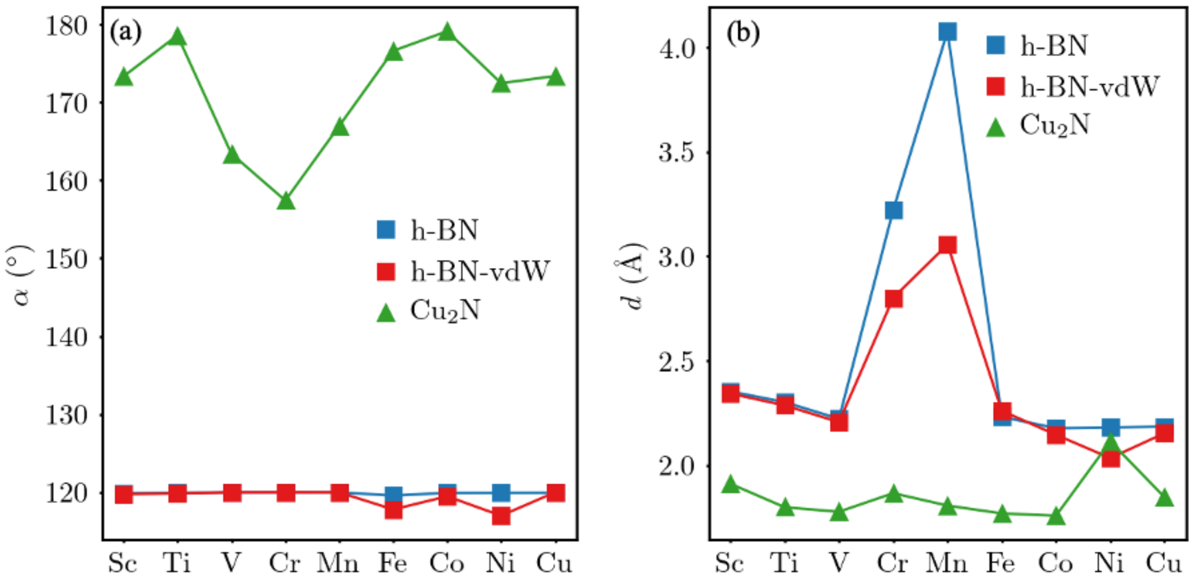


FIG. 7. Relaxed geometrical properties of top-stacked adatoms on $Cu_2N$, h–BN and h–BN-vdW. (a) B–N–B and Cu–N–Cu bond angles and (b) Distance between the adatom and nitrogen.
